# Supplementary material for: Optical Gaze Tracking with Spatially-Sparse Single-Pixel Detectors
Source: arXiv:2009.06875 source file (2021-02-02)
Supplement: Supplementary file 1 [file appendix.tex]

%!TEX root = script.tex

\small
